# Supplementary material for: A Hopfieldian View-based Interpretation for Chain-of-Thought Reasoning
Source: arXiv:2406.12255 source file (2024-06-18)
Supplement: Supplementary file 1 [file appendix-date-understanding-prompt.tex]

\begingroup
\begin{table*}[!ht]

    \centering
    \small
    \begin{tabular}{p{0.8\linewidth}}
        \toprule
        \underline{\textbf{\textsc{Prompt for Date Understanding}}} \\
        \vspace{-2mm}
        \textbf{Q:} 2015 is coming in 36 hours. What is the date one week from today in MM/DD/YYYY? \\
        \vspace{-1mm}
        \textbf{A:} \hl{If 2015 is coming in 36 hours, then it is coming in 2 days. 2 days before 01/01/2015 is 12/30/2014, so today is 12/30/2014. So one week from today will be 01/05/2015.} So the answer is 01/05/2015. \\
        \vspace{0mm}
        \textbf{Q:} The first day of 2019 is a Tuesday, and today is the first Monday of 2019. What is the date today in MM/DD/YYYY? \\
        \vspace{-1mm}
        \textbf{A:} \hl{If the first day of 2019 was Tuesday, then 01/01/2019 was a Tuesday. Today is the first monday, would be six days later. So today is 01/07/2019.}  So the answer is 01/07/2019.\\
        \vspace{0mm}
        \textbf{Q:}  The concert was scheduled to be on 06/01/1943, but was delayed by one day to today. What is the date 10 days ago in MM/DD/YYYY? \\
        \vspace{-1mm}
        \textbf{A:} \hl{One day after 06/01/1943 is 06/02/1943, so today is 06/02/1943. 10 days before today is 05/23/1943.} So the answer is 05/23/1943. \\
        \vspace{0mm}
        \textbf{Q:} It is 4/19/1969 today. What is the date 24 hours later in MM/DD/YYYY? \\
        \vspace{-1mm}
        \textbf{A:} \hl{Today is 04/19/1969. 24 hours later is one day after today, which would be 04/20/1969.} So the answer is 04/20/1969. \\
        \vspace{0mm}
        \textbf{Q:} Jane thought today is 3/11/2002, but today is in fact Mar 12, which is 1 day later. What is the date 24 hours later in MM/DD/YYYY? \\
        \vspace{-1mm}
        \textbf{A:} \hl{Today is 03/12/2002. So the date 24 hours later will be 03/13/2002.} So the answer is 03/13/2002. \\
        \vspace{0mm}
        \textbf{Q:} Jane was born on the last day of Feburary in 2001. Today is her 16-year-old birthday. What is the date yesterday in MM/DD/YYYY? \\
        \vspace{-1mm}
        \textbf{A:} \hl{The last day of February is the 28th, so Jane was born on 02/28/2001. Today is her 16-year old birthday, so today is 02/28/2017. So yesterday was 02/27/2017.} So the answer is 02/27/2017. \\
        \bottomrule
    \end{tabular}
    \label{tab:appendix-date-understanding-prompt}
    \caption{Few-shot exemplars for full chain of thought prompt for Date Understanding.}
\end{table*}
\endgroup
